# Supplementary material for: Get Your Vitamin C! Robust Fact Verification with Contrastive Evidence
Source: arXiv:2103.08541 source file (2021-03-15)
Supplement: Supplementary file 1 [file gen_examples.tex]

\begin{table*}[t]
\centering
\small
  \begin{tabular}{p{1cm}|p{13cm}}
\toprule
Claim    &  Stephen Bruner was born on October 18 , 1984 .   \\
\cmidrule{2-2} 
$s_{t-1}$ & Stephen Bruner ( born October 19 , 1984 ) , better known by his stage name Thundercat , is an American multi-genre bass player , producer and singer from Los Angeles , California .\\
\cmidrule{2-2} 
Output & Stephen Bruner ( born October 19, 1984 ), better known by his stage name Thundercat, is an American multi-genre bass player, producer and singer from Los Angeles, California.\\
\cmidrule{2-2}
$s_t$ & Stephen Bruner ( born October 19 , 1984 ) , better known by his stage name Thundercat , is an American multi-genre bass player , producer and singer from Los Angeles , California .\\
\midrule

Claim    &     \\
\cmidrule{2-2} 
$s_{t-1}$ & \\
\cmidrule{2-2} 
Output & \\
\cmidrule{2-2} 
$s_t$ & \\
\midrule

\bottomrule
\end{tabular}
\caption{Example outputs of the BART-base } \label{tab:gen_}
\end{table*}
