# Supplementary material for: Get Your Vitamin C! Robust Fact Verification with Contrastive Evidence
Source: arXiv:2103.08541 source file (2021-03-15)
Supplement: Supplementary file 2 [file gen_res.tex]

\begin{table*}[!h]
\centering
\small
    \resizebox{1\columnwidth}{!}{%
\begin{tabular}{l|l|ccc|cccc|c|c}
\toprule
Target & Model   	 & ROUGE1 & ROUGE2 & BLEU & KEEP & ADD & DEL & SARI & BLEURT & $f_{\mathrm{verdict}}$ \\
\midrule
\multirow{2}{*}{Revision} & T5	    	    & 83.98  & 77.63 & 47.46 & 72.61	& 13.32 & 43.04 & 42.99 & 0.38 & 64.52 \\
 & BART   	& 91.07	 & 85.23 & 54.86 & 75.36	& 18.31 & 47.95 & 47.21 & 0.67 & 76.26 \\
\midrule
\multirow{2}{*}{Claim} & T5 &  56.09 & 35.19 & 13.95 & 44.36 & 20.59 & 87.54 & 50.83 & -0.12 & 75.39  \\
& BART &                            62.28 & 40.38 & 16.14 & 52.91 & 23.62 & 91.37 & 55.97 & 0.16 & 85.83 \\

\bottomrule

\end{tabular}
    }
    \caption{Additional scores for the generation tasks, including ROUGE metrics and all three components of the SARI score. The rest of the metrics are copied from \tabref{tab:res_gen}. } \label{tab:app_gen}
\end{table*}
